# Supplementary material for: Investigating dissociation pathways of nitrobenzene via mega-electron-volt ultrafast electron diffraction
Source: arXiv:2308.03996 source file (2023-08-08)
Supplement: Supplementary file 1 [file sm_dissociation.tex]

\begin{figure}
    \centering
    \includegraphics[scale=0.37]{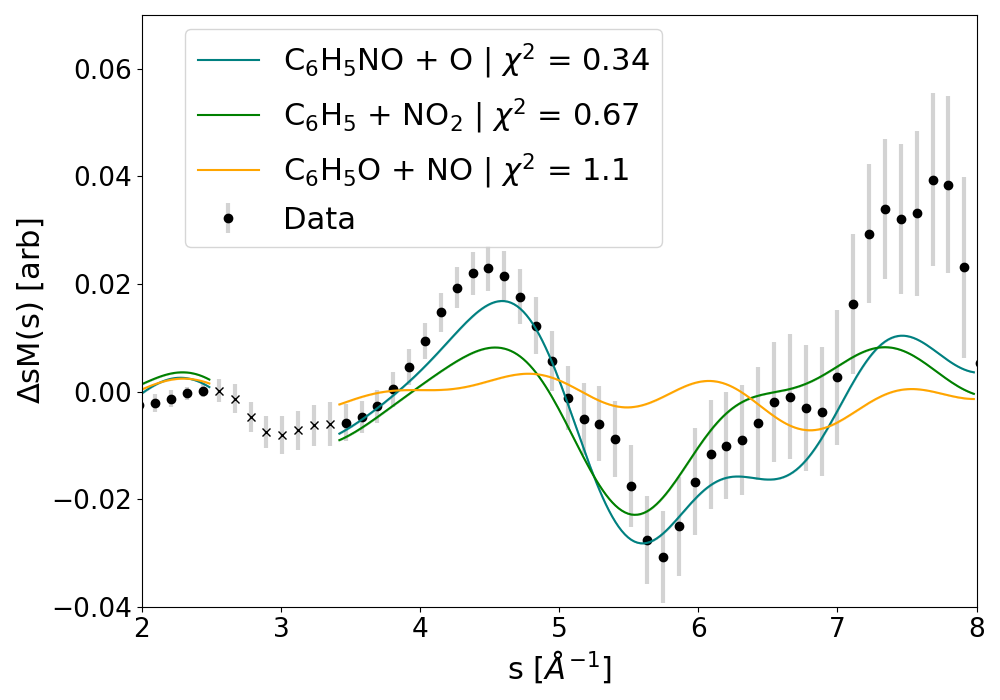}
    \caption{We show the agreement between the averaged measured \dsms{} after the signal has equilibrated and the simulated dissociative states.}
    \label{fig:diss_fit}
\end{figure}

Previous photolysis studies observed NO, \notwo, and O dissociation after nano or microseconds~\cite{Galloway.photolysisREMPI.1993, Galloway.LIF.1994, Lin.NOrempi.2007}.
When comparing simulations of these dissociative states with our averaged measured \dsms{} we observed poor agreement between the simulations and data.
Here we calculated the expected \dsms{} by splitting the molecule into its fragments and calculating the ground state geometry using Firefly QC package~\cite{Granovsky.Firefly.2022}, which is derived from the GAMESS (US)~\cite{Schmidt.GAMESS.1993} source code.
These \dsms{} calculations are thus based on a single geometry.
We observe that these simulations have poor agreement with the observed data, Fig.~\ref{fig:diss_fit}, except for \nsbz{} which has a very similar configuration to the S0 state.
The similarities between these simulations makes it difficult for us to distinguish between them.
However, since Saalbach \textit{et al.} did not observe any time-dependent fragmentation within the 100~ps \cite{Saalbach.photoelectron.2021} when searching for dissociative ions we do not expect to observe \nsbz.
We also note that when fitting with two final states we found that the combination of hot S0 and T1 had the best agreement with data, suggesting that it's unlikely we see both S0 and a dissociative state.
